# Supplementary material for: The Energy Cost of Controlling Mesoscopic Quantum Systems
Source: arXiv:1509.00914 source file (2015-09-03)
Supplement: Supplementary file 1 [file supp_mat_e_cost_qc_short.pdf]

# Supplemental Material: The Energy Cost of Controlling Mesoscopic Quantum Systems

Jordan M. Horowitz[1] and Kurt Jacobs[1,2]
[1]Department of Physics, University of Massachusetts at Boston, Boston, MA 02125, USA and
[2]Hearne Institute for Theoretical Physics, Louisiana State University, Baton Rouge, LA 70803, USA

In this supplemental material, we derive the minimum power required to coherently control a quantum system. This bound follows from a second-law-like inequality for the entropy production in an arbitrary quantum Markov process [1, 2]. We also define precisely the term "weak-coupling Hamiltonian" and compare our bound to the nonadiabatic entropy production rate.

*Minimum work bound.—* Our scenario is a pair of quantum systems $\mathcal{S}$, the controlled system, and $\mathcal{A}$, the auxiliary controller, with respective Hilbert spaces $\mathcal{H}_\mathcal{S}$ and $\mathcal{H}_\mathcal{A}$ and density matrices $\rho$ and $\chi$. These systems are weakly coupled through the Hamiltonian

$$\mathcal{H}(t) = H_\mathcal{S} + H_\mathcal{A} + V(t), \tag{1}$$

where $H_\mathcal{S}$ and $H_\mathcal{A}$ are, respectively, the system and auxiliary Hamiltonians, and $V \ll H_\mathcal{S}, H_\mathcal{A}$ is the weak interaction. Each subsystem weakly interacts with its own distinct environment, so that we can model the dynamics of the density matrix $\tau$ for the joint system $\mathcal{S} \oplus \mathcal{A}$ using the Lindblad master equation [3, 4]

$$\dot{\tau} = -\frac{i}{\hbar}[\mathcal{H}(t), \tau] + \sum_{i=1}^{N} \mathcal{D}^i_\mathcal{S}(\tau) + \mathcal{D}_\mathcal{A}(\tau) \equiv \mathcal{L}(\tau), \tag{2}$$

where the $\{\mathcal{D}^i_\mathcal{S}\}_{i=1}^N$ represent the environmental noise processes on the system and $\mathcal{D}_\mathcal{A}$ models the auxiliary's thermal reservoir at temperature $T$. The weak coupling of $\mathcal{S}$ and $\mathcal{A}$ ensures that when we combine $\mathcal{S}$ and $\mathcal{A}$ they do not affect each other's interaction with their own surroundings. Thus, the $\{\mathcal{D}^i_S\}$ operate solely on $\mathcal{H}_S$ without perturbing $\mathcal{A}$, and similarly $\mathcal{D}_A$ operates on $\mathcal{H}_A$. Furthermore, each noise process $\mathcal{D}^i_S$ has an invariant state $\pi^i$, given as $\mathcal{D}^i_\mathcal{S}(\pi^i) = 0$, while the auxiliary's noise, being thermal, has the equilibrium density matrix $\pi^{\rm eq}_\mathcal{A} \propto e^{-H_\mathcal{A}/T}$ as a fixed point in $k_{\rm B} = 1$ units.

Control is implemented by designing the coupling between $\mathcal{S}$ and $\mathcal{A}$ so that in the steady state $\tau^{\rm ss}$ – given as the solution of $\mathcal{L}(\tau^{\rm ss}) = 0$ – $\mathcal{S}$'s density matrix is $\rho^* = {\rm Tr}_\mathcal{A}[\tau^{\rm ss}]$.

Systems that satisfy a master equation, as in Eq. (2), obey a second-law-like inequality for the irreversible entropy production rate [1–3]

$$\begin{aligned}\Sigma = -\sum_{i=1}^{N} &{\rm Tr}[\mathcal{D}^i_\mathcal{S}(\tau)(\ln\tau - \ln\pi^i)] \\ &- {\rm Tr}[\mathcal{D}_\mathcal{A}(\tau)(\ln\tau - \ln\pi^{\rm eq}_\mathcal{A})] \geq 0.\end{aligned} \tag{3}$$

The sum is positive, since each term is individually positive. This follows because each term is the time-variation of a quantum relative entropy with respect to a quantum Markov process [5]. Specifically, imagine for the moment that the evolution of $\tau$ was generated by just one noise source: $\dot{\tau} = \mathcal{D}^i_\mathcal{S}(\tau)$. Then the time-variation of the quantum relative entropy $D(\tau||\pi^i) = {\rm Tr}[\tau\ln\tau - \tau\ln\pi^i]$ under this equation of motion, remembering that $\mathcal{D}^i_\mathcal{S}(\pi^i) = 0$, would be

$$\dot{D}^i(\tau||\pi^i) = {\rm Tr}[\mathcal{D}^i_\mathcal{S}(\tau)(\ln\tau - \ln\pi^i)] \leq 0. \tag{4}$$

The inequality is a result of the monotonicity of the quantum relative entropy under completely-positive, trace-preserving quantum maps [5]. Extending this observation to each term in Eq. (3), we conclude it is the sum of positive terms.

Our goal is to derive a bound on $\Sigma$ – which will imply the minimum power requirements – that only depends on $\mathcal{S}$ and its surroundings $\{\mathcal{D}^i_\mathcal{S}\}$, irrespective of the auxiliary. That way our bound will apply to any control. We start by observing that $\Sigma$ is at least as great as the entropy production due to just $\mathcal{S}$'s environment,

$$\Sigma \geq -\sum_{i=1}^{N} {\rm Tr}[\mathcal{D}^i_\mathcal{S}(\tau)(\ln\tau - \ln\pi^i)], \tag{5}$$

utilizing Eq. (4) for the auxiliary's thermal noise. This bound still depends on $\mathcal{A}$ through the joint density matrix $\tau$. However, we can again rely on the monotonicity of the relative entropy to coarse grain or trace over the auxiliary, which as a completely-positive, trace-preserving operation will decrease the relative entropy to

$$\Sigma \geq -\sum_{i=1}^{N} {\rm Tr}[\mathcal{D}^i_\mathcal{S}(\rho)(\ln\rho - \ln\pi^i)]. \tag{6}$$

The last step is to interpret the entropy production $\Sigma$ in terms of the energetics. Energy is driven into the system by each noise process $\dot{E}^i(\rho) = {\rm Tr}[\mathcal{D}^i_\mathcal{S}(\rho)H_\mathcal{S}]$, which is exhausted into $\mathcal{A}$'s thermal reservoir as heat

$$\dot{Q}_\mathcal{A} = -{\rm Tr}[\mathcal{D}_\mathcal{A}(\chi)H_\mathcal{A}] = T{\rm Tr}[\mathcal{D}_\mathcal{A}(\chi)\ln\pi^{\rm eq}_\mathcal{A}]. \tag{7}$$

The first law for the rate of change of the total energy then reads

$$\dot{E}(\tau) = \sum_{i=1}^{N} \dot{E}^i(\rho) - \dot{Q}_\mathcal{A} + \dot{W}, \tag{8}$$

where $\dot{W}$ is the work that is supplied to the auxiliary to affect the control. Thus, the entropy production in

Eq. (3) can alternatively be expressed as

$$\Sigma = -\mathrm{Tr}[\mathcal{L}(\tau)\ln\tau] + \sum_{i=1}^{N}\mathrm{Tr}[\mathcal{D}^i_{\mathcal{S}}(\tau)\ln\pi^i] + \frac{1}{T}\left[\sum_{i=1}^{N}\dot{E}^i(\rho) + \dot{W} - \dot{E}(\tau),\right], \tag{9}$$

using the quantum master equation [Eq. (2)] and the cyclic property of the trace.

Combining Eqs. (9) and (6), we find, after a simple rearrangement, a bound on the work rate

$$\dot{W} \geq \sum_{i=1}^{N} T\dot{S}^i_{\mathcal{S}}(\rho) - \dot{E}^i(\rho) + \dot{E}(\tau) - \dot{S}(\tau) \tag{10}$$

where $\dot{S}^i_{\mathcal{S}}(\rho) = -\mathrm{Tr}[\mathcal{D}^i_{\mathcal{S}}(\rho)\ln\rho]$ is the time variation of the system's von Neumann entropy due to $\mathcal{D}^i_{\mathcal{S}}$, and $\dot{S}(\tau) = -\mathrm{Tr}[\mathcal{L}(\tau)\ln\tau]$ is the variation of the system-plus-auxiliary von Neumman entropy.

To arrive at our main results [Eq. (2) of the main text], we specialize to the steady state where $\dot{E}(\tau^{\mathrm{ss}}) = \dot{S}(\tau^{\mathrm{ss}}) = 0$, leading to

$$\dot{W} \geq \sum_{i=1}^{N} T\dot{S}^i_{\mathcal{S}}(\rho^*) - \dot{E}^i(\rho^*) = -\sum_{i=1}^{N}\dot{F}^i_{\mathcal{S}}(\rho^*) \tag{11}$$

after identifying the rate of decrease in the system's free energy $\dot{F}^i_{\mathcal{S}}(\rho^*)$ due to its environmental noise. If instead, we desire to force the system through a specified evolution $\rho^*(t)$ during the time interval $t = 0$ to $\theta$, we then integrate Eq. (10) over this interval,

$$W \geq \int_0^\theta \sum_{i=1}^{N} T\dot{S}^i_{\mathcal{S}}[\rho^*(t)] - \Delta\dot{E}^i[\rho^*(t)]dt + \Delta E(\tau) - T\Delta S(\tau). \tag{12}$$

The term $\Delta F(\tau) = \Delta E(\tau) - T\Delta S(\tau)$ represents the free energy added to the system and auxiliary along the evolution during the time interval. Now, if the evolution is periodic, then $\Delta F(\tau) = 0$. Otherwise, we observe this added free energy is stored in the composite system and can in principle be recovered. Therefore, it does not contribute to the irretrievable work cost, and the minimum work cost (or dissipated heat) is

$$\begin{aligned} W_{\min} &= \int_0^\theta \sum_{i=1}^{N} T\dot{S}^i_{\mathcal{S}}[\rho^*(t)] - \Delta\dot{E}^i[\rho^*(t)]dt \\ &= -\int_0^\theta \sum_{i=1}^{N}\dot{F}^i_{\mathcal{S}}[\rho^*(t)]dt. \end{aligned} \tag{13}$$

consistent with the discussion following Eq. (2) in the main text.

*Definition of weak-coupling Hamiltonian.*— A weak coupling Hamiltonian, $V$, is any coupling Hamiltonian between the system and auxiliary that does not change appreciably the energy levels or eigenstates of the system, and naturally includes the trivial case in which the systems are not coupled at all. Since such a Hamiltonian allows arbitrary control of the system at a timescale slow compared to the system's internal dynamics, without changing the dynamics accessible with $V$ we can include a term that is a Hamiltonian only for the system, and which is sufficiently weak. We can also include an arbitrary Hamiltonian for the auxiliary, and this final inclusion provides the cleanest definition of $V$, since we do not need to distinguish between Hamiltonians that include a nonzero coupling and those that contain no coupling. Naturally the Hamiltonian $H_{\mathcal{A}}$ in the main text subsumes any auxiliary Hamiltonian that one might include as part of the weak-coupling Hamiltonian $V$. With these definitions out of the way, we can write an arbitrary weak coupling Hamiltonian as

$$V = V_{\mathcal{S}} + V_{\mathcal{SA}} + V_{\mathcal{A}}, \tag{14}$$

where $V_{\mathcal{S}}$ acts only on the system, $V_{\mathcal{SA}}$ may act on both the system and the auxiliary, and $V_{\mathcal{A}}$ acts only on the auxiliary. Since $V_{\mathcal{A}}$ does not change the system Hamiltonian at all, it is unconstrained. Since $V_{\mathcal{S}}$ does act on the system, the weak-coupling condition requires that

$$||V_{\mathcal{S}}|| \ll ||H_{\mathcal{S}}||, \tag{15}$$

where $H_{\mathcal{S}}$ is the system Hamiltonian and $||\cdot||$ denotes the $L_2$ norm (for example). The Hamiltonian $V_{\mathcal{SA}}$ acts on both the system and the auxiliary. Weak coupling requires that for any given state of the auxiliary, the Hamiltonian acting on $\mathcal{S}$ is small compared to $H_{\mathcal{S}}$. Thus choosing an arbitrary basis for $\mathcal{A}$ denoted by $\{|n\rangle\}$, we can break $V_{\mathcal{SA}}$ into the subblocks that act on $\mathcal{S}$ in the subspace defined by each of the $|n\rangle$:

$$V_{\mathcal{SA}} = \sum_n V^{(n)}_{\mathcal{SA}} \otimes |n\rangle\langle n|. \tag{16}$$

The condition for weak-coupling is then

$$||V^{(n)}_{\mathcal{SA}}|| \ll ||H_{\mathcal{S}}||, \qquad \forall n. \tag{17}$$

Finally, note that since an arbitrary shift in the energy of either system is irrelevant to the dynamics, the norms that appear above can be replaced by norms minimized over shifts of the overall energy. That is, in the expressions above we can replace a norm $||G||$ for any operator $G$ by

$$\min_{\alpha\in\mathbb{R}} ||G - \alpha I||, \tag{18}$$

where $I$ is the identity operator.

*Comparison with nonadiabatic entropy production.*— For a quantum system perturbed away from a nonequilibrium steady state, the nonadiabatic entropy production [6–8] has been identified as a useful thermodynamic

quantifier of irreversibility:

$$\begin{aligned}\Sigma^{\mathrm{na}} &= -\partial_s D(\tau_s||\tau^{\mathrm{ss}})\big|_{s=t} \\ &= -\sum_{i=1}^{N} \mathrm{Tr}[\mathcal{D}^i_{\mathcal{S}}(\tau)(\ln\tau - \ln\tau^{\mathrm{ss}})] \\ &\qquad - \mathrm{Tr}[\mathcal{D}_{\mathcal{A}}(\tau)(\ln\tau - \ln\tau^{\mathrm{ss}})].\end{aligned} \tag{19}$$

While the nonadiabatic entropy production resembles the irreversible entropy production rate in Eq. (3), they differ importantly in the reference state. For the nonadiabatic entropy production, the reference state is the global steady state $\tau^{\mathrm{ss}}$, by comparison the irreversible entropy production is measured in reference to the steady states of the individual noise processes.

[1] H. Spohn and J. L. Lebowitz, in *Advances in Chemical Physics: For Ilya Prigogine*, Vol. 38, edited by S. A. Rice (John Wiley & Sons, Hoboken, NJ, 1978).
[2] R. Alicki, M. Horodecki, P. Horodecki, and R. Horodecki, Open Sys. & Information Dyn. **11**, 205 (2004).
[3] H.-P. Breuer and F. Petruccione, *The Theory of Open Quantum Systems* (Oxford University Press, Oxford, 2007).
[4] K. Jacobs, *Quantum Measurement Theory and its Applications* (Cambridge University Press, Cambridge, 2014).
[5] T. Sagawa and M. Ueda, Phys. Rev. Lett. **100**, 080403 (2008).
[6] S. Yukawa, "The Second Law of Steady State Thermodynamics for Nonequilibrium Quantum Dynamics," (2001), arXiv:0108421v2.
[7] T. Sagawa, in *Lectures on quantum computing, thermodynamics and statistical physics*, Kinki University Series on Quantum Computing, Vol. 8, edited by M. Nakahara (World Scientific New Jersey, 2013).
[8] B. Gardas and S. Deffner, "Thermodynamics universality of quantum carnot engines," (2015), arXiv:1503.03455.
